# Supplementary material for: Bidisperse ring polymers: topological glass to stacking
Source: arXiv:2305.10812 ancillary file (2023-05-18)
Supplement: Supplementary file 1 [file supplemental.pdf]

# Supplementary Information
# Bidisperse ring polymers: topological glass to stacking

Projesh Kumar Roy,[1,2,*] Pinaki Chaudhuri,[1,2,†] and Satyavani Vemparala[1,2,‡]

[1] *The Institute of Mathematical Sciences, C.I.T. Campus, Taramani, Chennai 600113, India*
[2] *Homi Bhabha National Institute, Training School Complex, Anushakti Nagar, Mumbai – 400094, Maharashtra, India*

(Dated: May 18, 2023)

* projeshkr@imsc.res.in
† pinakic@imsc.res.in
‡ vani@imsc.res.in

# S.I. MODEL AND METHODS

## A. Model

For our study, we consider 400 non-concatenated ring polymers, where each polymer has 100 monomers (a total of 40,000 particles), and performed molecular dynamics (MD) simulation. The system size is chosen to be sufficiently large such that there are no self-interactions due to periodic boundary conditions, i.e., box length at any direction at equilibrium is larger than the diameter of an ideal 100-mer ring. Similar to our previous work [1], we have modeled various interactions between the monomers based on Kremer-Grest (KG) bead-spring model [2–4], which consists of– (a) Weeks-Chandler-Anderson (WCA) potential [5] (Eqn. 1), representing pairwise non-bonded interactions between any two monomers $\{ij\}$ separated by a distance of $r_{ij}$, (b) finitely extensible non-linear elastic (FENE) potential [2] (Eqn. 2), representing bonded interactions between two sequential monomers $\{ij\}$ in a polymer chain separated by a distance of $d_{ij}$, and (c) Kratky-Porod angular potential [6, 7] (Eqn. 3), which controls the stiffness of the rings by constraining the central angle $\theta$ between three sequential monomers $\{ijk\}$ in a polymer chain. The force-field equations are given below and force-field parameters are listed in table S.1. We have used reduced unit formalism to represent all variables used in this paper. The unit of time is defined as $\tau = \sigma\sqrt{(}m/\mathrm{k_B}T)$, where $m$ is the mass of the monomers and $\mathrm{k_B}$T is the unit of energy. The mass of each monomer was taken to be 1.0. The energies and length scales are in terms of $k_BT$ and $\sigma$.

$$U_{\mathrm{WCA}}(r_{ij}) = \begin{cases} 4\epsilon\left[\left(\frac{\sigma}{r_{ij}}\right)^{12} - \left(\frac{\sigma}{r_{ij}}\right)^{6} + \frac{1}{4}\right] & r_{ij} \leq 2^{1/6}\sigma \\ 0 & r_{ij} > 2^{1/6}\sigma \end{cases} \tag{1}$$

$$U_{\mathrm{FENE}}(d_{ij}) = \begin{cases} -0.5\kappa R_0^2 \ln\left[1 - \left(\frac{d_{ij}}{R_0}\right)^2\right] & d_{ij} < R_0 \\ \infty & d_{ij} \geq R_0 \end{cases} \tag{2}$$

$$U_{\mathrm{Angle}}(\theta) = K_\theta[1 - cos(\theta - \pi)] \tag{3}$$

The force field parameters are listed in Table 1.

TABLE S.1. Force-field parameters: Monomers of A-type belong to ring polymers with stiffness $K_\theta^A$ =1.0 – 10.0 and B-type belongs to ring polymers with $K_\theta^B$ = 20.0. The force-field parameters are represented in their usual symbols, see Ref. 1 for detailed descriptions.

| Parameter | Value |
|---|---|
| $\sigma_{AA} = \sigma_{BB} = \sigma_{AB}$ | 1.0 $\sigma$ |
| $\epsilon_{AA} = \epsilon_{BB} = \epsilon_{AB}$ | 1.0 $\mathrm{k_B}T$ |
| $\kappa_{AA} = \kappa_{BB}$ | 30.0 $\mathrm{k_B}T/\sigma^2$ |
| $R_{0,AA} = R_{0,BB}$ | 1.5 $\sigma$ |
| $K_\theta^A$ | 1.0 $\mathrm{k_B}T$, 5.0 $\mathrm{k_B}T$, 10.0 $\mathrm{k_B}T$ |
| $K_\theta^B$ | 20.0 $\mathrm{k_B}T$ |

## B. Simulation details

Ring polymers with two different stiffness parameters, $K_\theta^A$ (flexible A-type) and $K_\theta^B$ (stiffer B-type) were mixed with different ratios to create a set of stiffness mixtures. The stiffness for the B-type rings is fixed at $K_\theta^B$ = 20.0, while $K_\theta^A$ was changed from 1.0–10.0. A similar equilibration procedure as in Ref. 1 was followed. The starting configurations of the systems were generated as a random distribution of rings at a very low density ($4 \times 10^{-5}$). Under periodic boundary conditions, the pressures of the systems were gradually increased upto the target pressure using a sufficiently small timestep of0.003, and subsequent equilibration MD simulations were run till the energy and density fluctuations stabilize (see Fig. S.1(a)(c)). Using the final equilibrated structures from each run, production runs of

$10^8$ steps were performed for each system using a time step of $0.006\tau$. The temperature ($T = 1.0$) and pressure ($P = 1.0$) of the systems were kept fixed using overdamped Nosé - Hoover chains thermostat [8, 9] and barostat [10] with coupling timescale $t_d = 1.0$. The variation of average potential energy and density as a function of A-type polymer concentration is shown in Fig. S.1(b)(d).

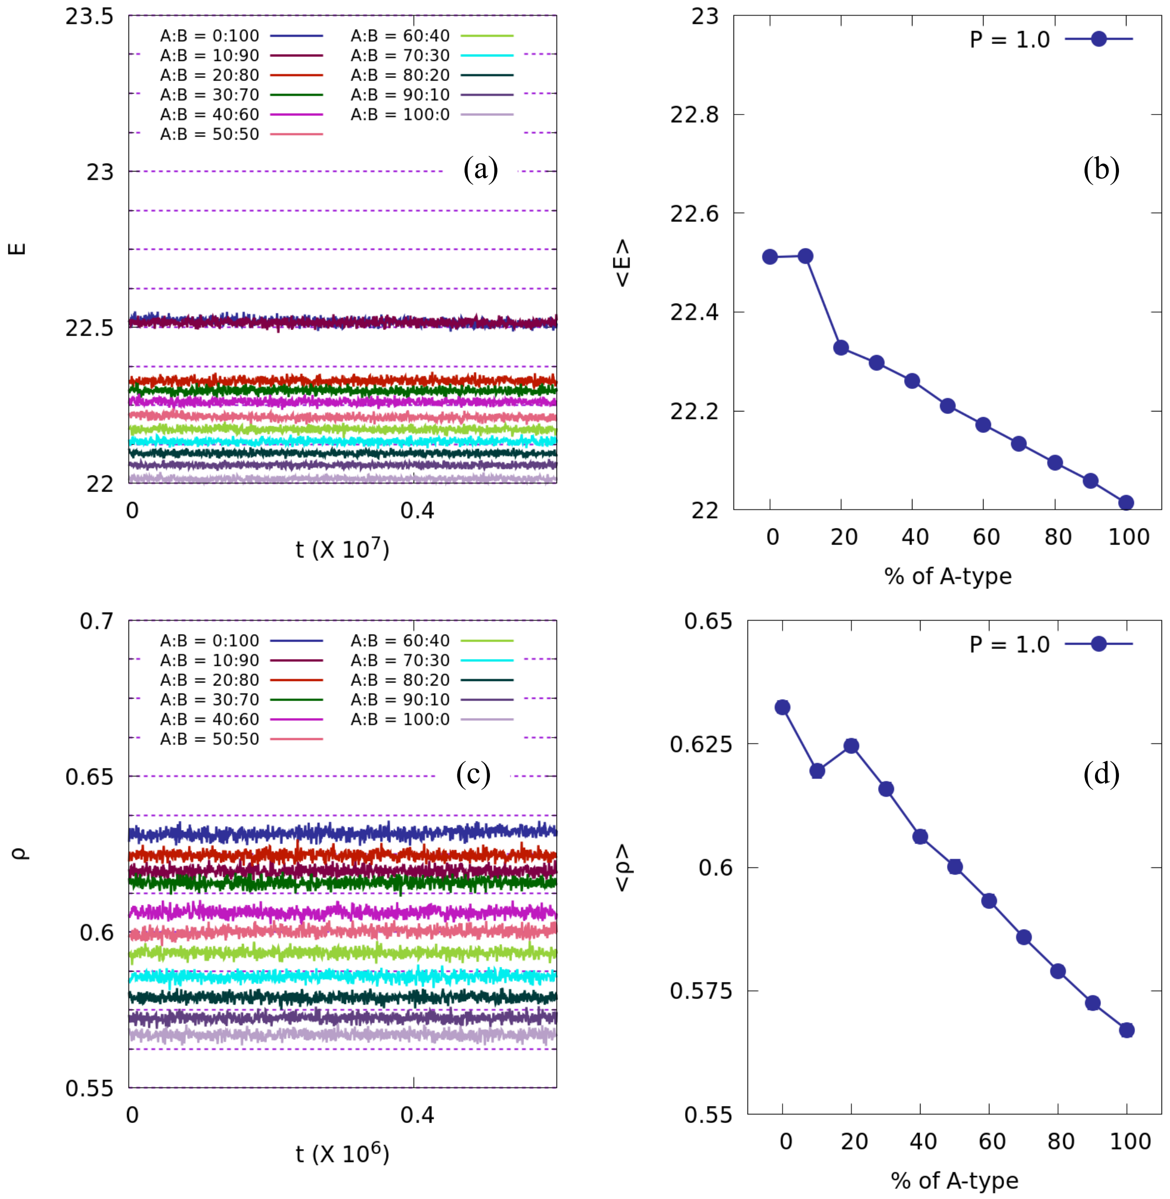


FIG. S.1. Variation of the (a) total potential energy per particle and (c) density at different concentrations of A-type ring for pressure $P = 1.0$. Corresponding average data are plotted in (b) and (d). All data in (b), and (d) are averaged over the last $10^7$ steps with 100 data points.

### C. Detection of stacking and clustering

To characterize the visible observed stacking behavior of the B-type rings, we use the algorithm by Poier *et al* [11, 12]. The methodology is as follows–first, the eigenvectors ($\mathbf{d}_{\text{min, i}}$) with the lowest eigenvalues are identified for the $i^{\text{th}}$ ring, which is assumed to be oriented almost perpendicularly to the minimal plane of the ring. Then, all the neighbor rings ($j$'s) are identified whose center-of-mass vectors ($\mathbf{r}_{\text{COM, ij}}$) are relatively parallel to the minimum eigen vector of $i^{\text{th}}$ ring, i.e., $\mathbf{d}_{\text{min, i}}.\mathbf{r}_{\text{COM, ij}}/(|\mathbf{d}_{\text{min, i}}||\mathbf{r}_{\text{COM, ij}}|) > 0.9$. The rings are further filtered to remove distant rings with a

stricter distance criterion, $|\mathbf{r}_{\text{COM, ij}}|_{\|} \leq 2.0$ and $|\mathbf{r}_{\text{COM, ij}}|_{\perp} \leq 2.0$. A matrix $M_{\text{st}}$ of size $R \times R$ can be constructed whose components $M_{\text{st}}(i, j) = 1$ in case $i^{\text{th}}$ and $j^{\text{th}}$ rings are stacked against each other, and zero otherwise. Self-stacking is excluded from this calculation.

## S.II. THERMODYNAMIC DATA

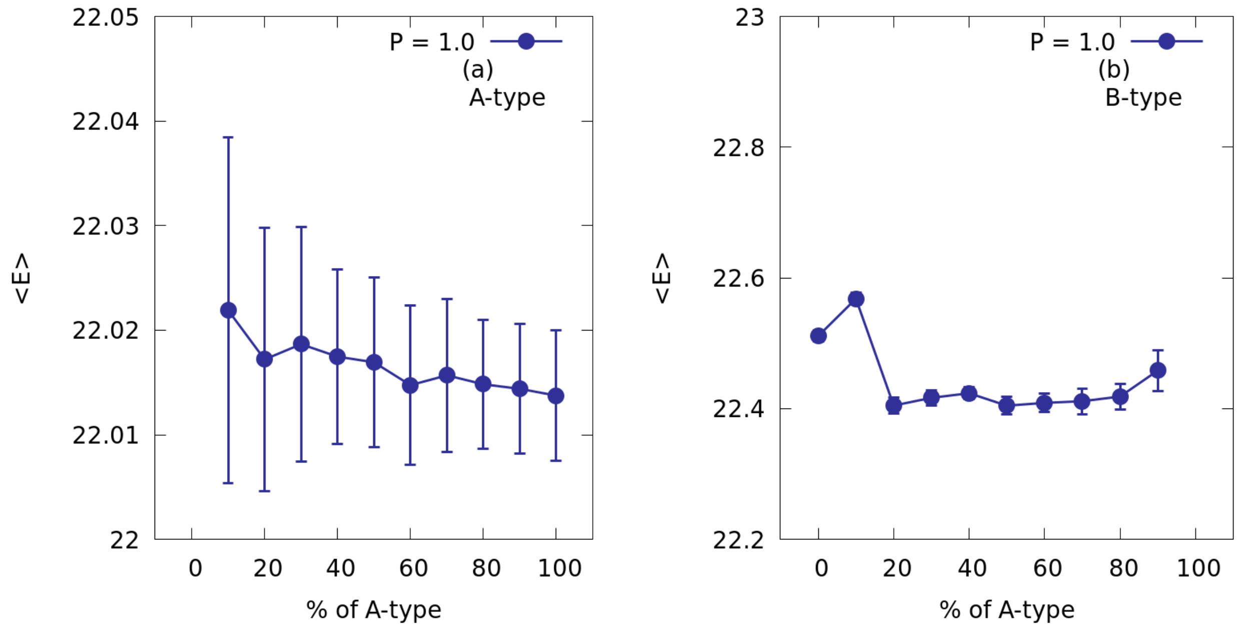


FIG. S.2. Variation of average potential energy per particle of (a) A-type rings and (b) B-type rings. (c) Relative density of A-type and B-type rings at different concentrations of A-type rings for pressure $P = 1.0$. All data in all plots are averaged over the last $10^7$ steps with 100 data points.

The total average energy ($\langle E \rangle$) of the equilibrated systems decreases with increasing concentration of A-type rings (Fig. S.1(a)(b)). Interestingly, $\langle E \rangle_{\text{B}}$ of the B-type rings decreases sharply around A-type:B-type=20:80 mixture (Fig. S.2(b)), while $\langle E \rangle_{\text{A}}$ of A-type rings remains more or less constant (Fig. S.2(a)).

## S.III. EFFECT OF VARYING $K_\theta^A$

The initial structure for $K_\theta^A = 5.0, 10.0$ are taken from the final equilibrated structure of A-type:B-type=80:20 case with $K_\theta^A = 1.0$. These structures are equilibrated and simulated under NPT conditions with the new stiffness parameters, using the same procedure as described in the earlier section. The sudden drop in the average number of unstacked B-type rings for $K_\theta^A = 10.0$ indicates competition for the depletion interaction emerges between A-type and B-type rings. Therefore, the critical value for clear phase separation in our binary mixture lies in between $5.0 \leq K_\theta^A \leq 10.0$.

## S.IV. CLUSTER SIZE DISTRIBUTION

In Fig. S.4(b), we show the distribution of the cluster sizes, which are normalized by the total available mass of the B-type rings in the mixture. With increasing the % of A-type rings, the distribution shifts to the right side of the plot, indicating that at large dilution, the entire system will form a single cluster. Although during our simulation time, we did not see the formation of a single cluster; from Fig. S.4(b) we predict that, at high dilution, a single cluster of stiff B-type rings is the eventual reality. To prove this, we manually prepare a single stack-cluster of equidistant B-type rings (center-of-mass distance $1.0\sigma$) to immerse it inside a sea of A-type rings with a total composition of A:B=90:10, and monitor its stability using MD simulations. The entire system was first packed inside a large box, and then slowly

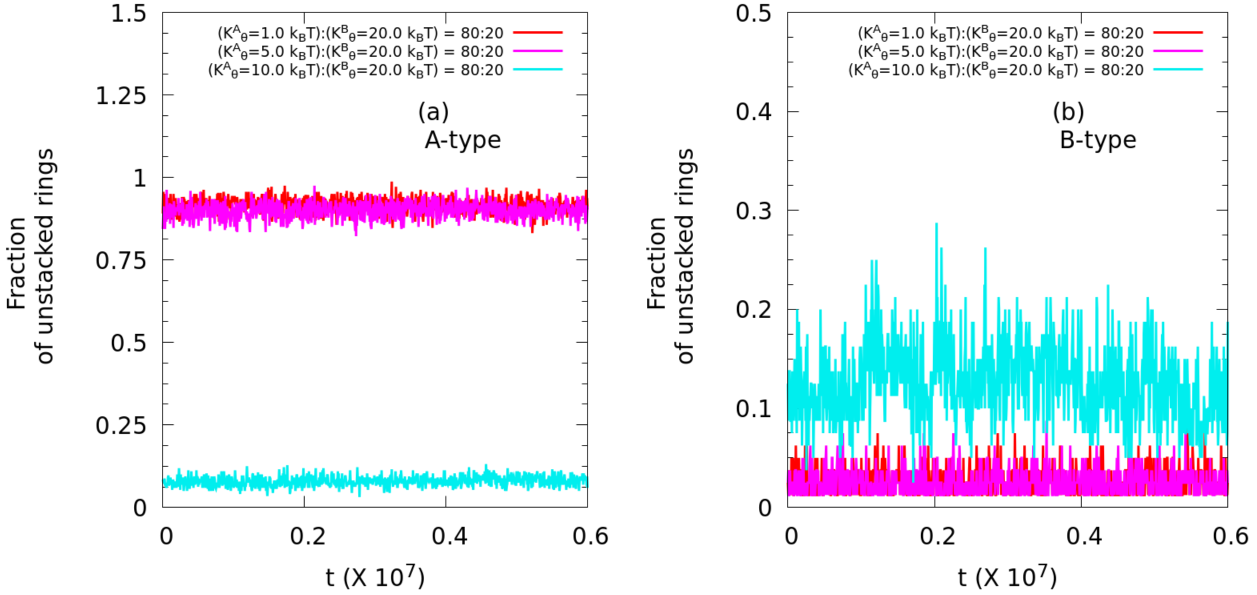


FIG. S.3. Variation of the average number of unstacked rings for (a) A-type rings with different $K_\theta^A$ values and (b) B-type rings for A-type:B-type=80:20 case.

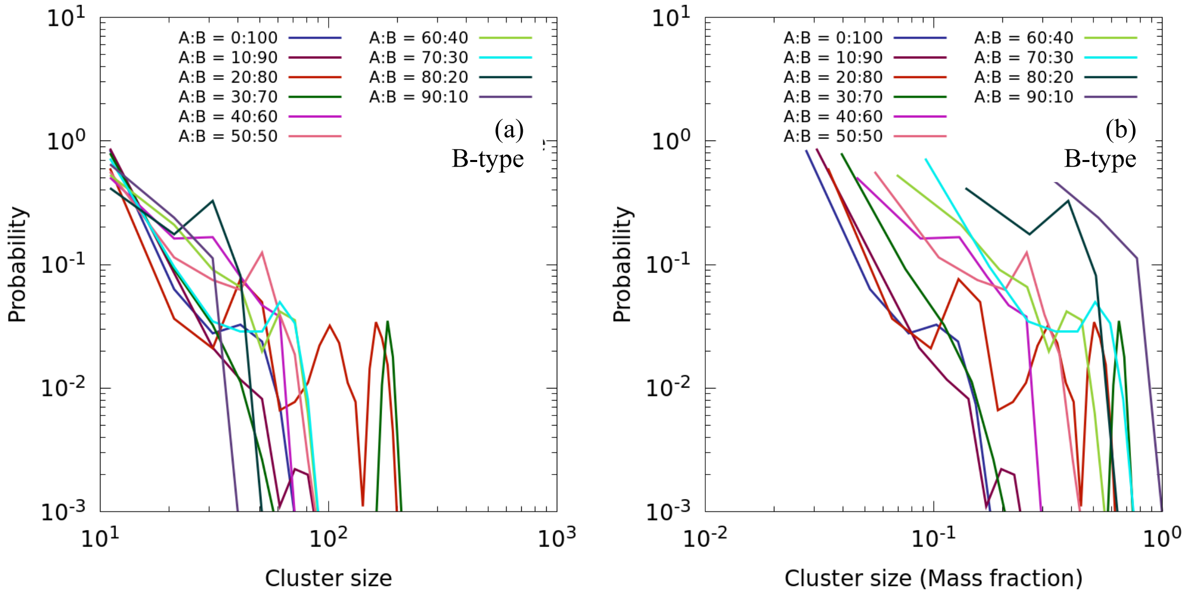


FIG. S.4. Histogram of the (a) cluster-size and (b) cluster-size normalized by the total number of available B-type rings, for B-type rings at different concentrations of A-type rings at pressure $P = 1.0$. All data are averaged over the last $10^7$ steps with 100 data points.

squeezed to achieve the expected density. Thus, the equilibration phase was performed in two steps; box-scaling under NVT conditions, and followed by MD simulation under NPT conditions. During the NVT simulation step of the equilibration phase, the box size is slowly scaled in a cyclic manner to achieve the targeted density. In between these cycles, the system is equilibrated as follows–(i) First, only the A-type rings are coupled with the thermostat for $10^4$ steps, during which B-type rings do not move. (ii) Then, only the B-type rings are minimized while holding the A-type rings fixed in their positions. In the last step, the interactions between A-type and B-type rings are removed temporarily during minimization and then again turned back on. In this way, the columnar structure of the B-type rings is well maintained during the box scaling, and at the same time, the energy of the total system was brought

down. Next, during the NPT step of the equilibration phase, only the A-type rings are coupled to the thermostat and barostat, while the B-type rings are simply dilated to maintain their geometry during box fluctuations.

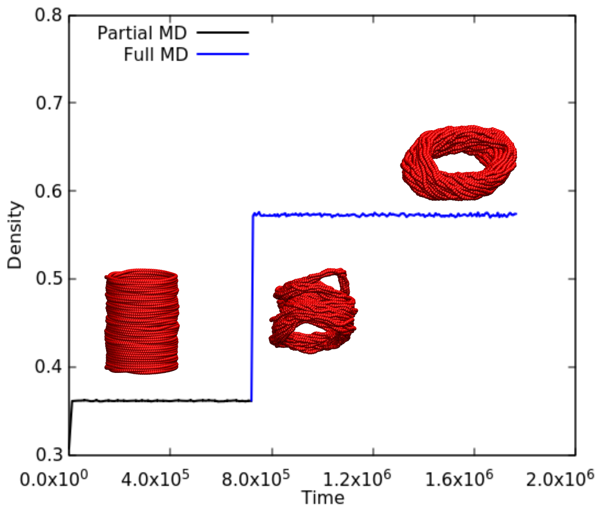


FIG. S.5. Structural rearrangement of a single stack-cluster of B-type rings inside A-type:B-type=90:10 system with time. The time axis is starting from the equilibration phase (NPT) and the subsequent production phase. In the inset, snapshots of the evolution of the single stack-cluster of B-type rings with time are shown.

After the partial relaxation of the system is complete, production MD steps were started where all constraints were removed. Now, both A-type and B-type rings were coupled to the thermostat and barostat to monitor the structural evolution of the ideal single column of B-type rings. We find that during the production MD phase, this column quickly collapses and takes a more compact form by increasing the peripheral entanglement in between the B-type rings (see Fig. S.5). This collapsed single stack-cluster remains quite stable during the production MD phase, which indicates that the single stack-cluster phase is, in fact, a stable state point of this binary mixture at a large dilution.

## S.V. THREADING ANALYSIS

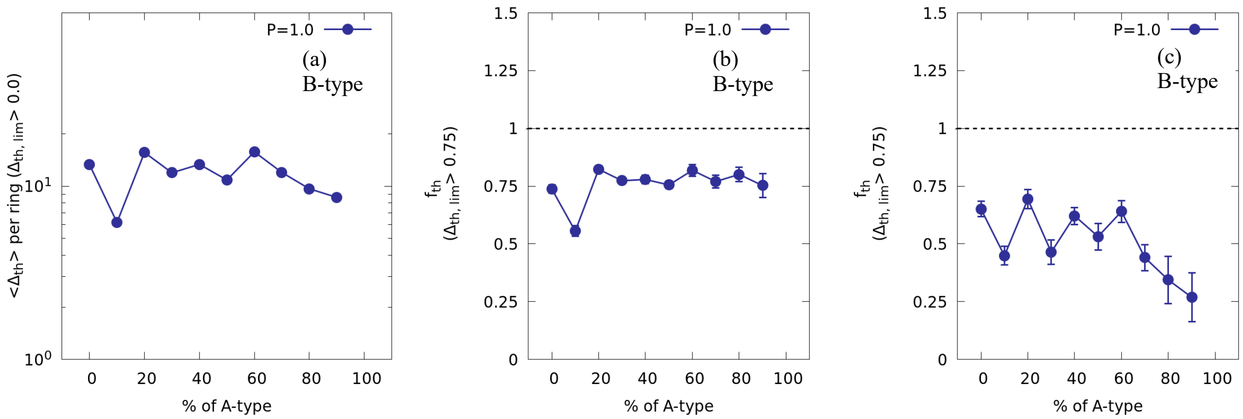


FIG. S.6. Variation of (a) $\langle \Delta_{\rm th} \rangle$ of B-type rings at different concentrations of A-type rings at pressure $P = 1.0$ at a coarse-grain level of 17 particles. The fraction of threaded rings ($f_{\rm th}$) with $\Delta_{\rm th,lim} > 0.75$ at a coarse-grained level of (b) 17 particles and (c) 4 particles are also plotted. All data in all plots are averaged over the last $10^7$ steps with 100 data points.

We further calculated the net quantity of self-threading inside the set of B-type rings in terms of an average

threading parameter ($\langle\Delta_{\rm th}\rangle$). For the details of the algorithm to determine $\langle\Delta_{\rm th}\rangle$, we refer to our previous publication in Ref. 1. Since the A-type rings do not participate in any kinetically significant threading, we discard all threading calculations involving A-type rings. We find that variation of the $\langle\Delta_{\rm th}\rangle$ of B-type rings follow no significant trend upto A-type:B-type $\sim$ 60:40 case, although, at very high % of A-type polymers, the slight decreasing trend is noticed (see Fig. S.6(a)). This data can be explained by dividing the threading effects into two parts, orthogonal and peripheral threading. Inside a single stack-cluster, the B-type rings tend to thread mainly along the periphery to maintain the columnar structure, which is expected to decrease the overlap of the minimal surface area of two B-type rings and subsequently decrease $\langle\Delta_{\rm th}\rangle$. However, at large concentrations of B-type rings, the stack-clusters often inter-penetrate each other in an orthogonal manner, which increases the threading parameter. Therefore, in the diluted regime, the effect of peripheral threading dominates over orthogonal threading, whereas in the concentrated regime, the opposite effect takes place. The competition between these two effects can only be seen clearly if one coarse-grains the topology of the rings. In the case of orthogonal threading, the total amount of entanglement would mildly change with coarse-graining, whereas peripheral threading will decrease it. Hence, we have degraded the topology of the rings up to 4 particles by periodically skipping 30 particles along the chain. As shown in Fig. S.6(c), the fraction of highly threaded rings (with $\Delta_{\rm th,lim} > 0.75$) clearly decreases with this method after A-type:B-type $\sim$ 60:40, which indicates that peripheral-threading dominates at larger dilution.

## S.VI. SUPPLEMENTARY MOVIES

- movie1.mp4 : Equilibrium trajectory corresponding to A:B=0:100 and $K_\theta^A = 1.0$ and $K_\theta^B = 20.0$.
- movie2.mp4 : Equilibrium trajectory corresponding to A:B=10:90 and $K_\theta^A = 1.0$ and $K_\theta^B = 20.0$.
- movie1.mp4 : Equilibrium trajectory corresponding to A:B=90:10 and $K_\theta^A = 1.0$ and $K_\theta^B = 20.0$.
- movie1.mp4 : Equilibrium trajectory corresponding to A:B=80:20 and $K_\theta^A = 10.0$ and $K_\theta^B = 20.0$..


[1] P. K. Roy, P. Chaudhuri, and S. Vemparala, Soft Matter **18**, 2959 (2022).
[2] K. Kremer and G. S. Grest, The Journal of Chemical Physics **92**, 5057 (1990), https://doi.org/10.1063/1.458541.
[3] J. D. Halverson, W. B. Lee, G. S. Grest, A. Y. Grosberg, and K. Kremer, The Journal of chemical physics **134**, 204904 (2011).
[4] J. D. Halverson, W. B. Lee, G. S. Grest, A. Y. Grosberg, and K. Kremer, The Journal of chemical physics **134**, 204905 (2011).
[5] J. D. Weeks, D. Chandler, and H. C. Andersen, The Journal of Chemical Physics **54**, 5237 (1971), https://doi.org/10.1063/1.1674820.
[6] M. Doi and S. Edwards, *The theory of polymer dynamics* (Oxford University Press, 1988).
[7] F. Guo, K. Li, J. Wu, L. He, and L. Zhang, Polymers **12**, 2659 (2020).
[8] S. Nosé, The Journal of Chemical Physics **81**, 511 (1984).
[9] G. J. Martyna, M. L. Klein, and M. Tuckerman, The Journal of Chemical Physics **97**, 2635 (1992).
[10] S. Nosé and M. Klein, Molecular Physics **50**, 1055 (1983).
[11] P. Poier, P. Bačová, A. J. Moreno, C. N. Likos, and R. Blaak, Soft Matter **12**, 4805 (2016).
[12] P. Poier, C. N. Likos, A. J. Moreno, and R. Blaak, Macromolecules **48**, 4983 (2015).
